# Supplementary material for: A linguistically-motivated evaluation methodology for unraveling model's abilities in reading comprehension tasks
Source: arXiv:2501.17569 source file (2025-01-29)
Supplement: Supplementary file 1 [file additional_analysis.tex]

\begin{table}[]
\resizebox{\columnwidth}{!}{%
\begin{tabular}{c|c|c|c|c|c|c|c|}
\cline{2-8}
                          & Rouge-L     & \% correct & $P(f2\mid S)$ & $P(f3\mid S)$ & $P(f4\mid S)$ & $P(f5\mid S)$ & $P(f6\mid S)$ \\ \hline
\multicolumn{1}{|c|}{S1}  & 0.80 - 0.92 & 100        & 0.35    & 0.44    & 0.26    & 0.55    & 0.53    \\ \hline
\multicolumn{1}{|c|}{S2}  & 0.54 - 0.68 & 43 - 56    & 0.38    & 0.47    & 0.32    & 0.65    & 0.61    \\ \hline
\multicolumn{1}{|c|}{all} & 0.69 - 0.82 & 71 - 82    & 0.37    & 0.46    & 0.29    & 0.59    & 0.57    \\ \hline
\end{tabular}%
}
\caption{Probability of having the $fi$ factor with \textbf{S1} the split of "easy" examples (where models agree and on the right answer), \textbf{S2} the other examples considered as "hard" and \textbf{all} on all the corpus.}
\label{tab:proba-factor}
\end{table}

Figure \ref{fig:proba-factor-agreement} shows that the probabilities of the presence of factors $f5$ and $f6$ vary the most. These factors start with a high probability in the subsets where the models disagree the most and consistently remain the most probable factors across all subsets.

\begin{figure}
 \begin{center}
  \includegraphics[width=0.5\textwidth]{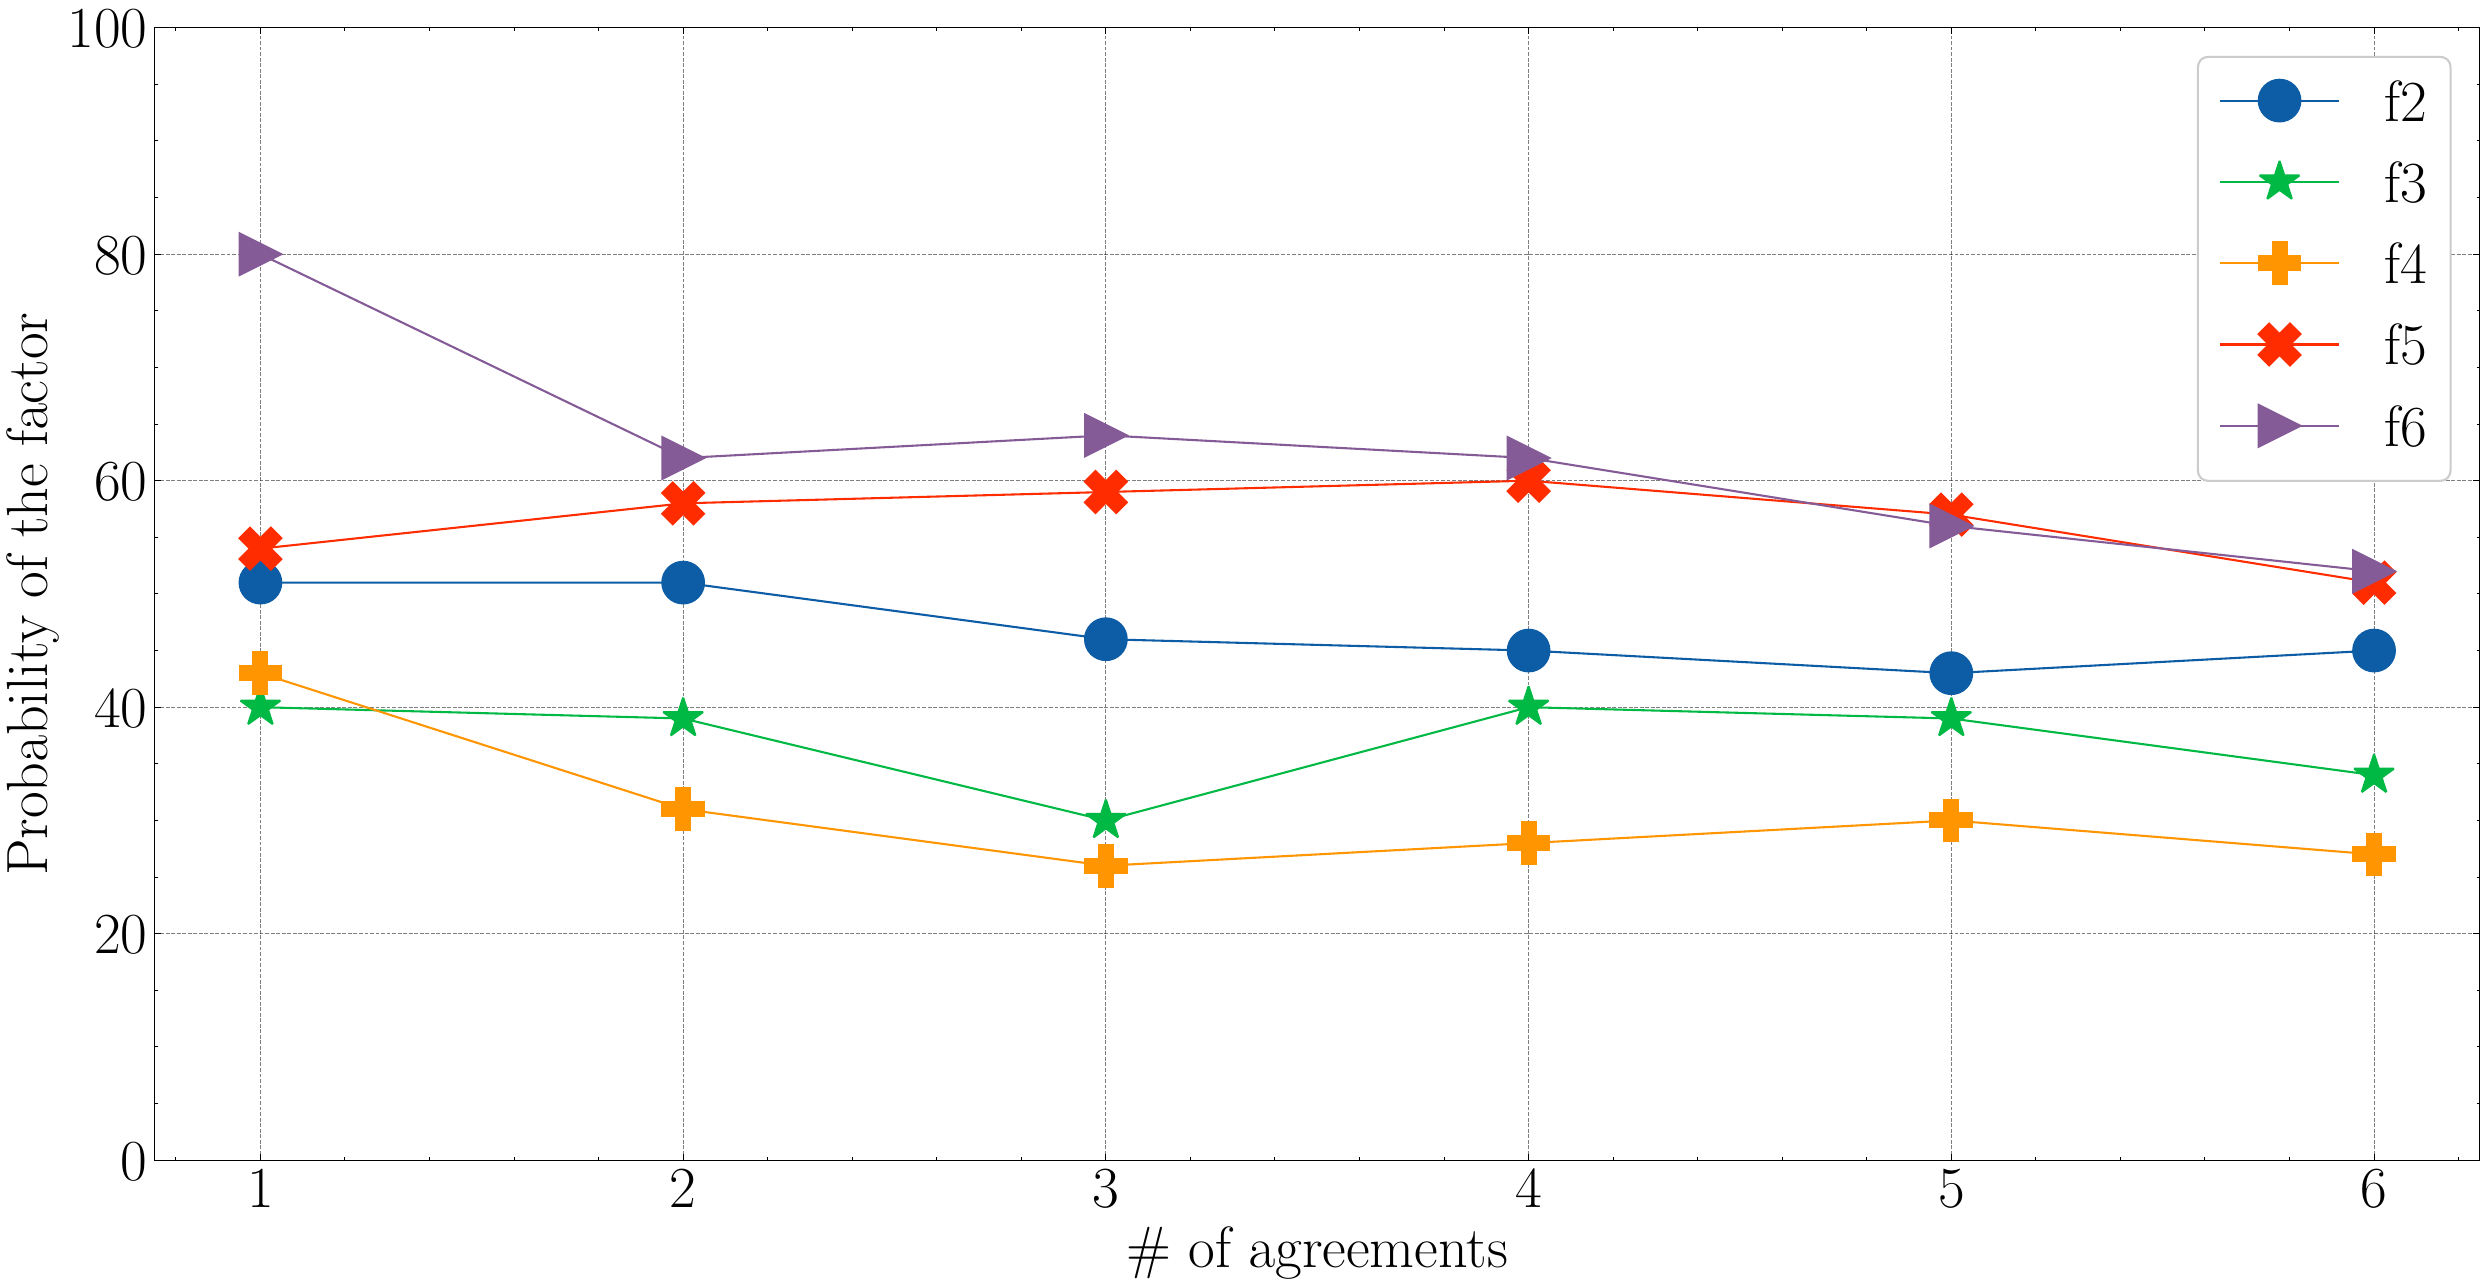} 
  \caption{Probability of having the $fi$ factor by split of the example according to the number of agreement between the models}
 \label{fig:proba-factor-agreement}
 \end{center}
 \end{figure}

 \begin{figure*}[h]
 \begin{center}
  \includegraphics[width=1\textwidth]{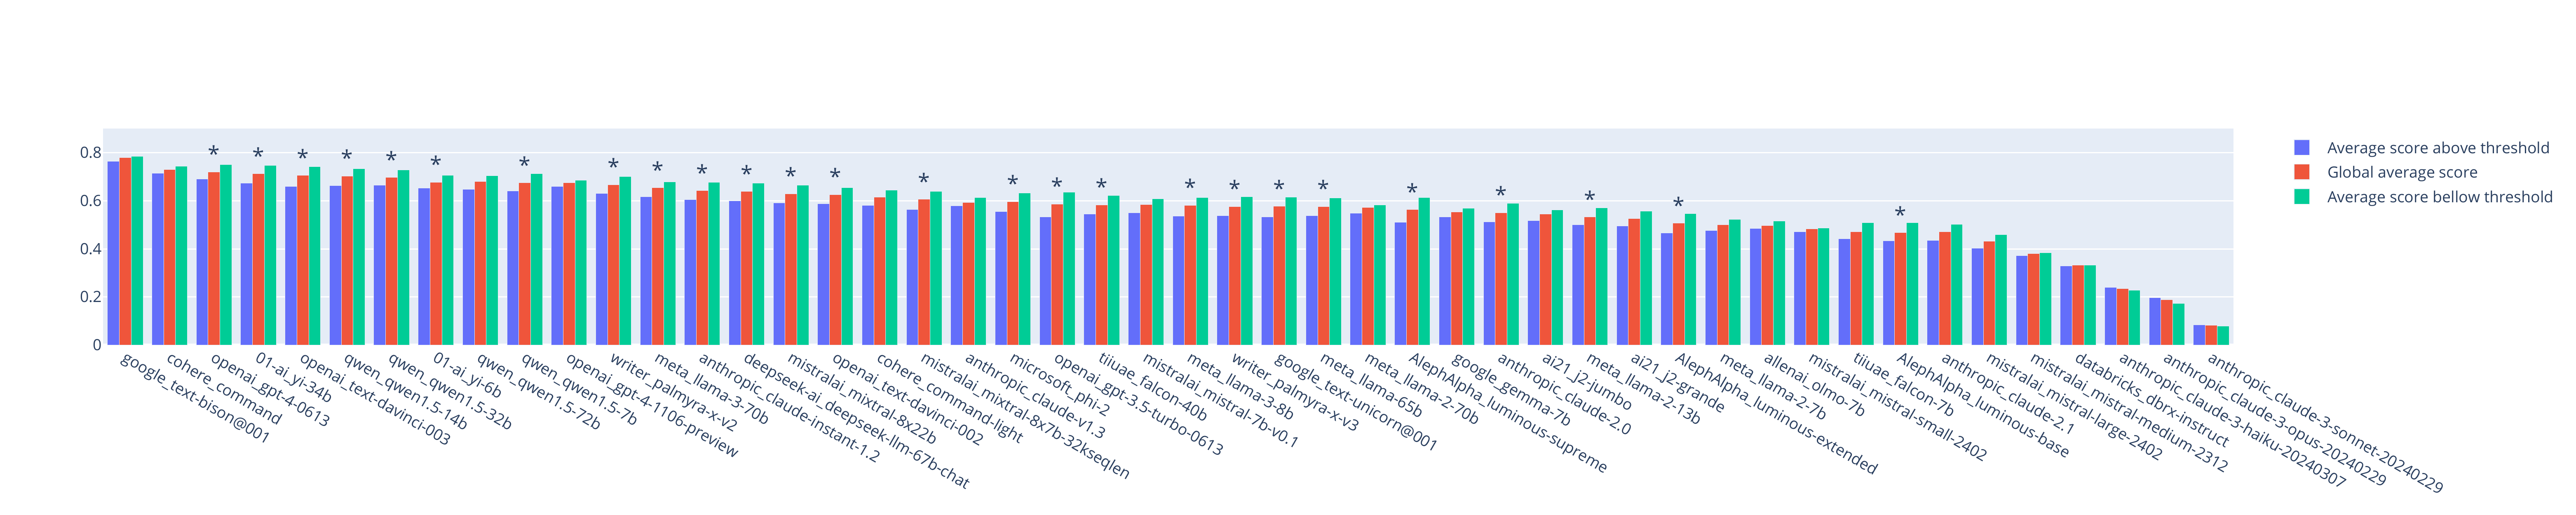} 
  \caption{Models F1 score on 3 partitions of the difficult subset of the evaluation corpus according to $f6$, "*" denotes a significant score difference}
 \label{fig:score_natural_qa_difficult}
 \end{center}
 \end{figure*}

 \begin{figure*}[h]
 \begin{center}
  \includegraphics[width=1.2\textwidth]{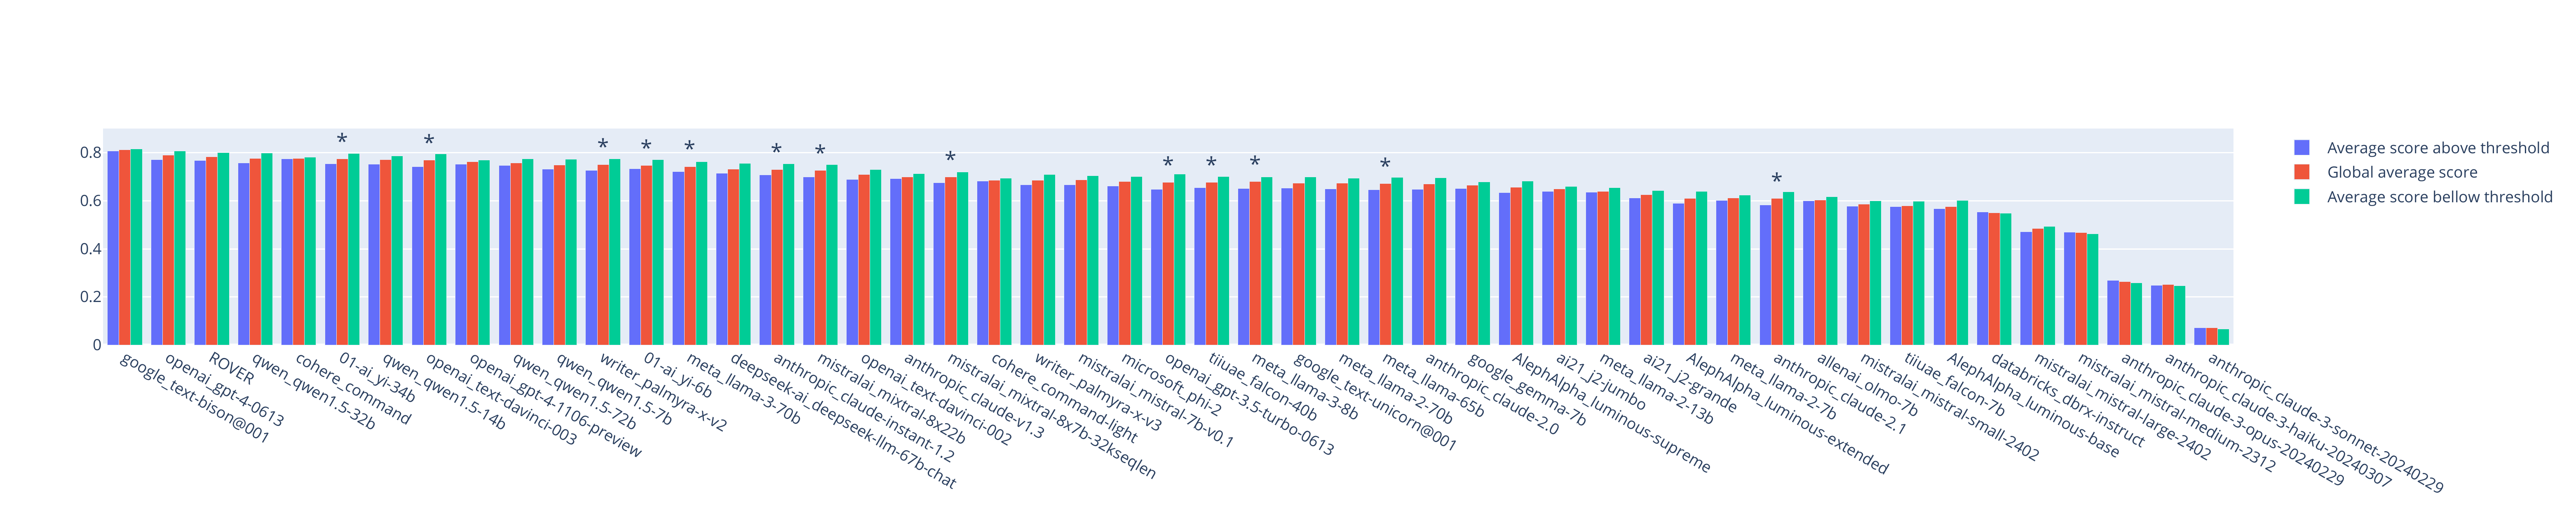} 
  \caption{Models F1 score on 3 partitions of the evaluation corpus according to $f6$, "*" denotes a significant score difference}
 \label{fig:score_natural_qa_all}
 \end{center}
 \end{figure*}

\begin{figure*}[h!]
 \begin{center}
  \includegraphics[width=1\textwidth]{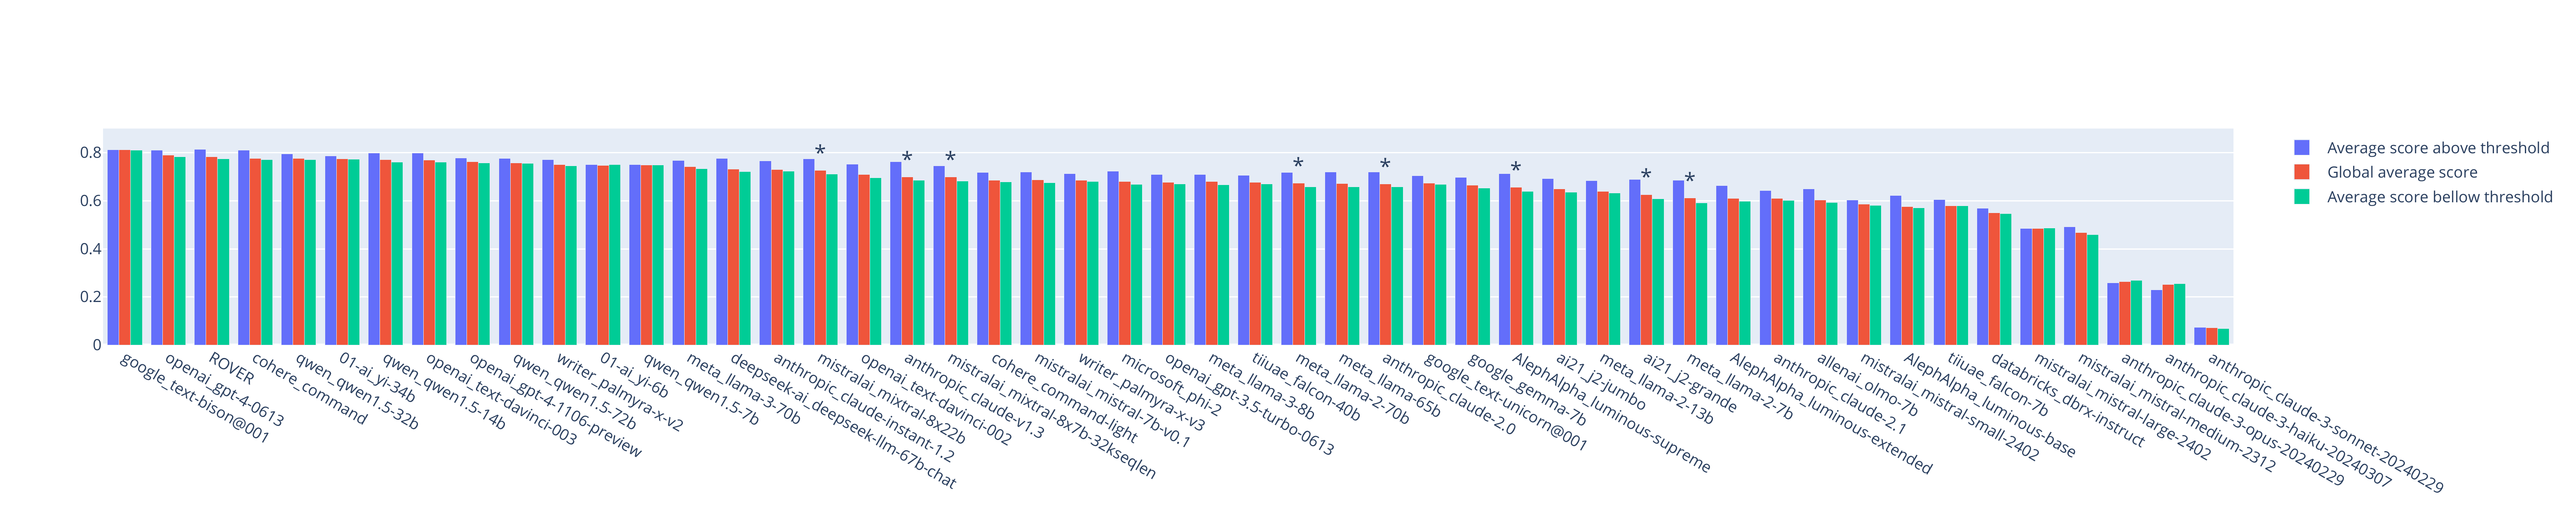} 
  \caption{Models F1 score on 3 partitions of the evaluation corpus according to $f5$, "*" denotes a significant score difference}
 \label{fig:score_natural_qa_fe_all}
 \end{center}
 \end{figure*}

\begin{table}[]
\resizebox{\columnwidth}{!}{%
\begin{tabular}{|c|cc|}
\hline
                                  & \multicolumn{2}{c|}{Factors}                   \\ \hline
models/factors                    & \multicolumn{1}{c|}{f5}          & f6          \\ \hline
size of Ef (\%)                   & \multicolumn{1}{c|}{80\%}        & 52\%        \\ \hline
google\_text-bison@001            & \multicolumn{1}{c|}{0}           & -2          \\ \hline
qwen\_qwen1.5-32b                 & \multicolumn{1}{c|}{-3}          & \textbf{-6} \\ \hline
meta\_llama-3-70b                 & \multicolumn{1}{c|}{-4}          & \textbf{-6} \\ \hline
mistralai\_mixtral-8x7b-32kseqlen & \multicolumn{1}{c|}{\textbf{-9}} & \textbf{-8} \\ \hline
meta\_llama-3-8b                  & \multicolumn{1}{c|}{-5}          & \textbf{-8} \\ \hline
google\_gemma-7b                  & \multicolumn{1}{c|}{-4}          & -4          \\ \hline
meta\_llama-2-7b                  & \multicolumn{1}{c|}{-8}          & -5          \\ \hline
mistralai\_mistral-large-2402     & \multicolumn{1}{c|}{1}           & \textbf{-6} \\ \hline
\end{tabular}%
}
\caption{Hard subset of naturalQA}
\label{tab:complex-naturalQA-hard}
\end{table}

\begin{figure*}[h]
 \begin{center}
  \includegraphics[width=1\textwidth]{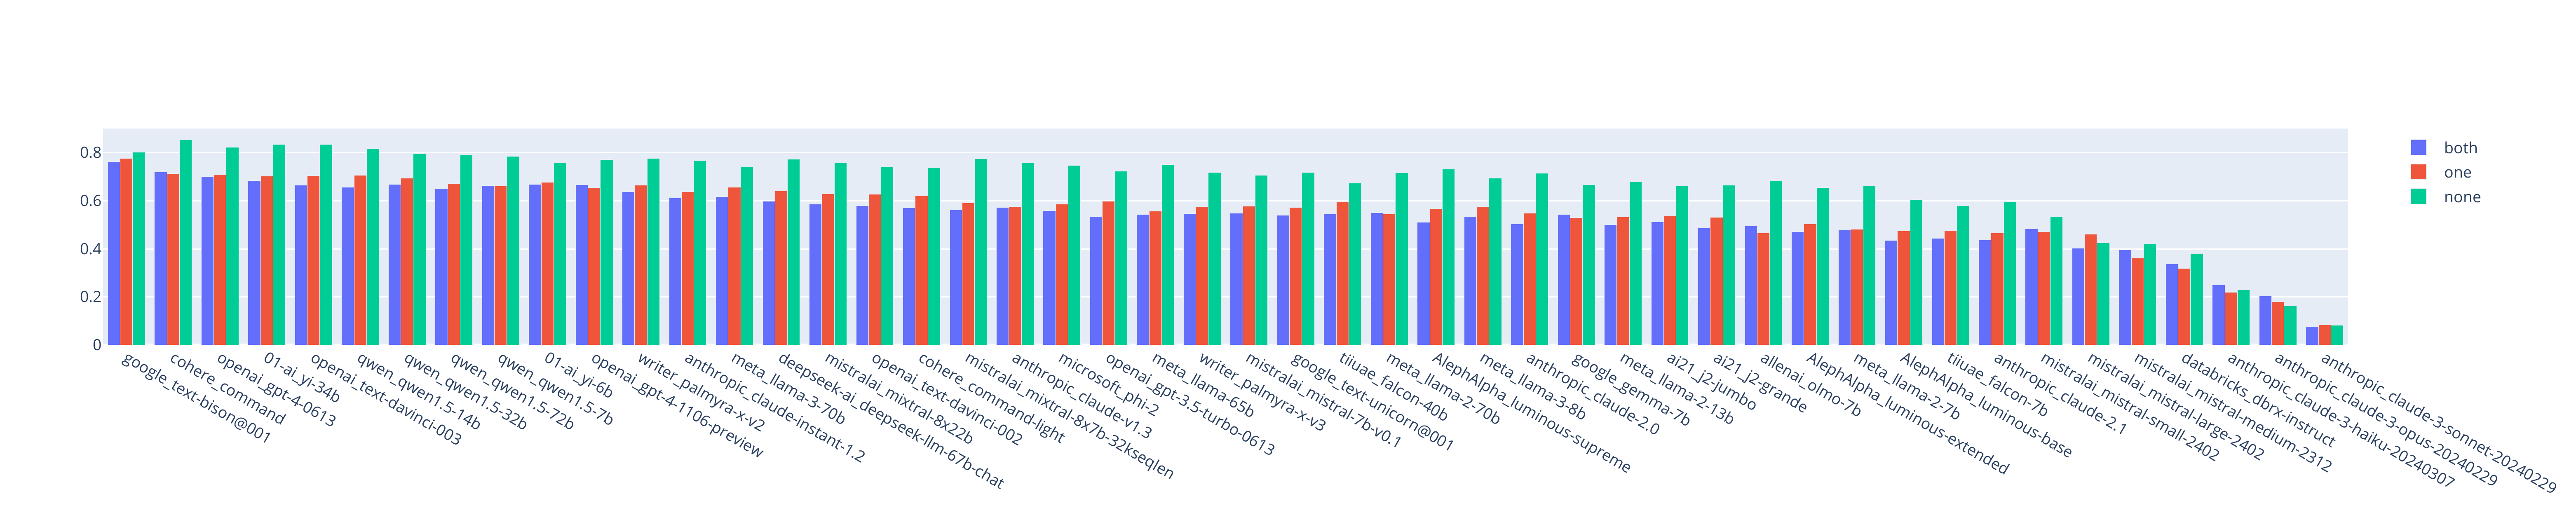} 
  \caption{Models F1 score on 3 partitions of the difficult subset of the evaluation corpus according to combinations of complexity factors $f5$ and $f6$}
 \label{fig:natural_qa_fe_entropy_hard}
 \end{center}
 \end{figure*}
